# Supplementary material for: Molecular dynamics characterization of the free and encapsidated RNA2 of CCMV with the oxRNA model
Source: arXiv:2408.03662 ancillary file (2024-08-07)
Supplement: Supplementary file 1 [file supp.pdf]

# Supplementary Material

## *Molecular dynamics characterization of the free and encapsidated RNA2 of CCMV with the oxRNA model*

Dr. Giovanni Mattiotti,[1] Manuel Micheloni,[2,3] Dr. Lorenzo Petrolli,[2,3] Prof. Samuela Pasquali,[1] Prof. Luca Tubiana,[2,3] and Prof. Raffaello Potestio[2,3]

[1]*Laboratoire Biologie Functionnelle et Adaptative, CNRS UMR 8251, Inserm ERL U1133, Université Paris Cité, 35 rue Hélène Brion, Paris, France*

[2]*Department of Physics, University of Trento, via Sommarive, 14 I-38123 Trento, Italy*

[3]*INFN-TIFPA, Trento Institute for Fundamental Physics and Applications, Trento, Italy*

## I. RNA2 SEQUENCE

1 GUAAUCCACG AGAGCGAGGU UCAAUCCCUU GUCGACUCAC GGGUCUCCAU CAGUUGAAAA

61 CAGUUUAUAC AUUUUCUUCU UGAUAUUUUU CUUCUUUACU UCCAUUAAUA UGUCUAAGUU

121 CAUUCCAGAA GGUGAGACUU ACCACGUUCC CUCAUUCCAA UGGAUGUUUG AUCAGACUCU

181 CGAAUCUGAC UCACACCAUG AUGAGGCGAU AUUCGUAACC GAAUCGAUUA AUGAAAGUGG

241 AGUUGAUACU UCUGUUGAAA UAACCGCAGA UGGCACGCUA GCAAGUUAUA UGCAUGCCGU

301 AAAGCCCCUA GUGGAGGAUG GUCUUCUGAA UCCCCCUUUU GAUCAAGCUA GAUGGGGUCU

361 UUGCUGCAAG AACGUCGUUG ACGUUUAUGA CGGGCUGCUC GGUUAUAGAC UCAUACCAAU

421 GGCUGAAGCC GCUAGAAUGU UGUACUUGGA AAUCGACGGU UCAUUCGUUG AUGAAUCUGA

481 GUGUGACGAU UGGCGGCCGG UAGAUACCUC UGAUGGUUUC ACCGAAGCAA UGUUUGAUGU

541 GAUGAAUGAG AUUCCUGGCG AGGAAACAAA AAAUACAUGC GCUUUAAGUC UUGAAGCUGA

601 AUCAAGGCAA GCUCCAGAAA CUUCCGAUAU GGUGCCGUCU GAAUAUACGU UGGCAGAUAG

661 GUACGUUACC ACCAGAGAGG AGUUCGCGUC UGUUGACUCG GAUUAUGACA UAUCCUUAAA

721 CCUGGUGAGC CCUGUGGAGU UCAGGGUGGG AGUGUGUGAA GACACAUACC GUCAUUCGGA

781 AGCUGAUGAU CCUACGAUGC CUCAAUAUCA CGAUAGGAUC AGUUUAAAAU CGCUGGAGGC

841 GGCUGGCCAU CACAUGUUAC CGACUCAUGC CUAUUUUGAC GACACUUACU ACCAGGCUUU

901 GGAAGAGCUA GGCGAUUAUA AUGUCGAUAU UAGUAAGUUG UCUGUCCGGC AGAGUGAUGU

961 UGAUUGGUAU CGUGACCCUG AAAAGUACUA UGAGCCUGAG UUAAGUAUAG GGUCAUUCCA

1021 ACGUAGAAUA GGUACGCAAA AGACGGUCCU UACCGCGUUA AAGAAACGGA ACGCUGACGU

1081 GCCUGAGUUA GCAGAUUCUG UUGAUAUUAA AAGAGUAGCC UGUGAAGUAG CUGAAAAAUU

1141 UAAACGGGCU UAUCUUAAUC AUUCCGGUAU AGGGCUGUUA GGGCAAAGUA UGGAUGUCAU

1201 GUCCAGAGGA CUUGAGUACC AUAAGAAAUG GAAAGACCAC AAAGACCUGA CUGGUGUGAC

1261 AGUUUUGUCU GAGAUUAAUU UGCAGAGGUA UCAGCACAUG AUAAAGUCUG AUAUUAAACC

1321 AGUUGUCUCG GAUACGUUAC ACCUCGAACG AGCUGUUGCU GCAACAAUAA CAUUUCAUGG

1381 UAAAGGAGUU ACUAGCUGCU UCUCACCAUA UUUUACGGCU UGUUUCGAGA AGUUUUCAAA

1441 AGCUUUAAAA UCAAGGUUUG UGGUCCCCAU AGGGAAGAUC UCCUCCCUGG AACUGAAAAA

1501 UGUUCCCCUC UCGAAUAAAU GGUUUCUUGA GGCGGAUUUG AGUAAGUUUG AUAAAUCUCA

1561 GGGUGAGCUU CAUCUUGAGU UCCAAAGAGA GAUAUUGUUG UCAUUGGGUU UUCCAGCCCC

1621 UUUGACUAAU UGGUGGUGUG AUUUCCAUAG GGAAUCUAUG CUAUCGGAUC CUCAUGCUGG

1681 AGUUAACAUG CCAGUUUCCU UUCAGCGUCG UACUGGUGAU GCUUUUACUU AUUUUGGGAA

1741 UACUUUGGUG ACUAUGGCCA UGAUGGCCUA UUGUUGCGAU AUGAACACCG UGGACUGUGC

1801 UAUCUUUUCC GGUGAUGAUU CUCUGUUAAU UUGUAAAAGU AAACCACAUC UGGAUGCUAA

1861 UGUUUUUCAA UCUCUGUUUA AUAUGGAAAU UAAAGUUAUG GACCCAAGUU UGCCAUACGU

1921 UUGUAGUAAG UUUCUUUUAG AAACUGAAAU GAAUAACUUG GUGUCUGUGC CUGAUCCUAU

1981 GAGAGAGAUA CAGAGACUGG CUAAGCGAAA GAUCAUCAAA UCGCCUGAGU UGUUAAGAGC

2041 CCACUUUGAG UCCUUUUGUG AUAGGAUGAA AUUCCUAAAC AAAUUGGAUG AAAAAAUGAU

2101 AAAUUUAUUA UGCAAGUUUG UGGCUCUCAA GUAUAAAAAA CCUGACGUUG AAAACGAUGU

2161 CAGAGUAGCC AUUGCUGCUU UCGGCUACUA CUCAGAAAAU UUCUUGAGAU UUUGCGAAUG

2221 UUAUGCGACU GAAGGGGUCA AUAUAUAUAA GGUAAAACAU CCCAUCACCC AGGAGUGGUU

2281 CGAGGCCUCU AGGGAUCGAG ACGGUGACUG GUUCCAUGAC UGGCGUAAUC CGAAGUUUCC

2341 CACUGCCUUA GAUAAGGUUU GGAGAUUCUU UGGAAAAUAC GCGAGAGAUG AUCCUAUGAA

2401 GCACAUAGAA GAGAGAGAUA GGAGACAUAG GCUUAAUCGA GCCAUGAAUU CUUCCUUGAA

2461 ACUUGCCUAU GAUCGUAGGA GUCUUAGUAA GGAUAAAGAA ACCGUUGCGU GGGUGCGUAA

2521 GACCCUUUCU AAAUAAUGUU GGUCACAUUU AAGACUUGUU UAGUCCACAU UAGGACUGGU

2581 UCUAACAGUU UCUUUAAACU GUAAUCGUCG UUGCGACGUU GGUUUGCUUA CAAGCAAUCA

2641 AGCUGCCUUU GAGUUUUACU CCUUGAACUC UUCAGAAGAA UUCUUCGGAA UUCGUACCAG

2701 UAUCUCACAU AGUGAGGUAA UAAGACUGGU GGGCAGCGCC UAGUCGAAAG ACUAGGUGAU

2761 CUCUAAGGAG ACCA

## II. FREELY-FOLDING STAGE

### A. RNA2 conformations

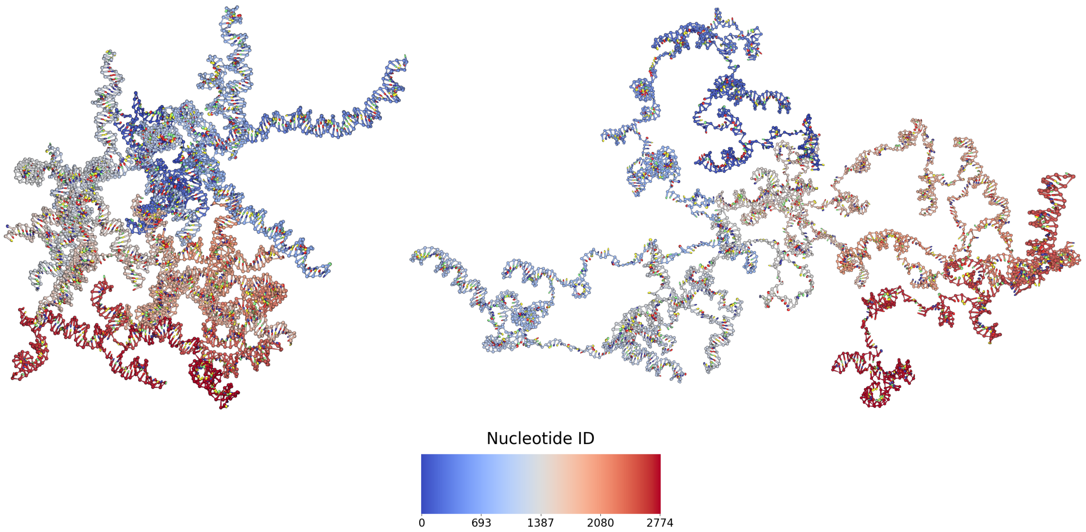


**Supplementary Figure S1**: (Example) snapshots of RNA2 conformations at (**left**) 0.5 M, and (**right**) 0.15 M, as a result of the freely-folding relaxation. The color code is associated with the nucleotide index.

## B. Distance matrices between (intra-replica, intra-concentration) contact maps

To quantify the variability in the secondary structures of RNA2, we defined a distance $d_{KM}$ between contact maps as follows: Given two Boolean contact maps $\{k_{ij}^{(1)}\}$, $\{k_{ij}^{(2)}\}$ associated with frames (1) and (2), the distance counts all contacts that are "true" in either (not both) frames - which is equivalent to a logical XOR criterion. The 2D matrices showing the values of $d_{KM}$ for each duple of frames within a given replica, and within all MD replicas per salt concentration, are shown in Fig. **S2** (0.15 M) and **S3** (0.5 M), and Fig. **S4** respectively. A hierarchical clustering based on an *average linkage* criterion was performed on the (intra-concentration) distance matrices of Fig. **S4** - dendrograms are shown in Fig. **S5** (0.15 M) and **S6** (0.5 M).

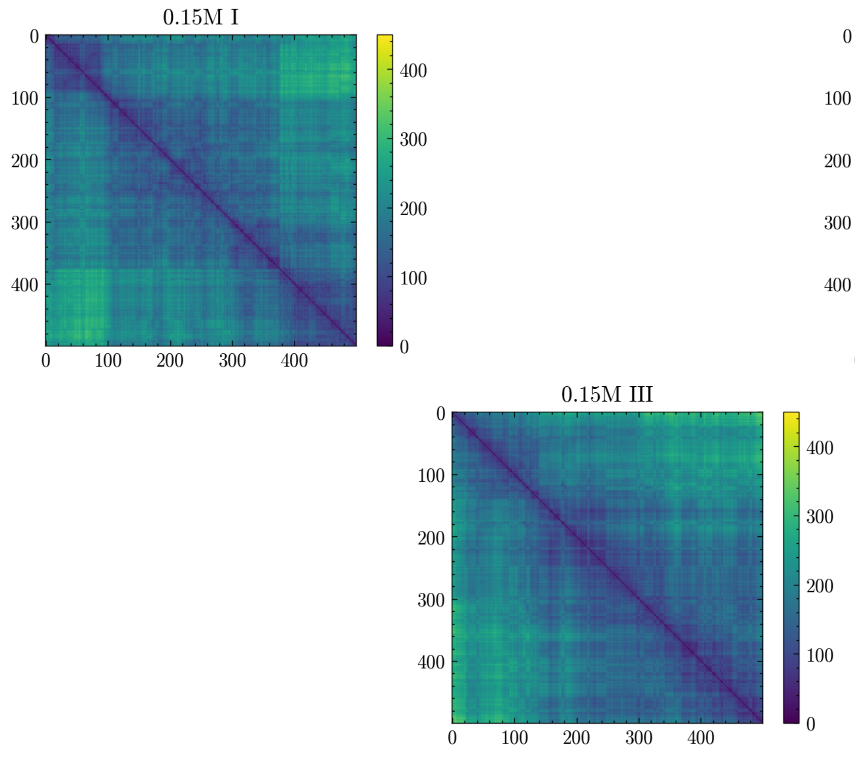


**Supplementary Figure S2**: 2D distance matrices ($d_{KM}$) between contact maps, associated with the freely-folding MD replicas at 0.15 M.

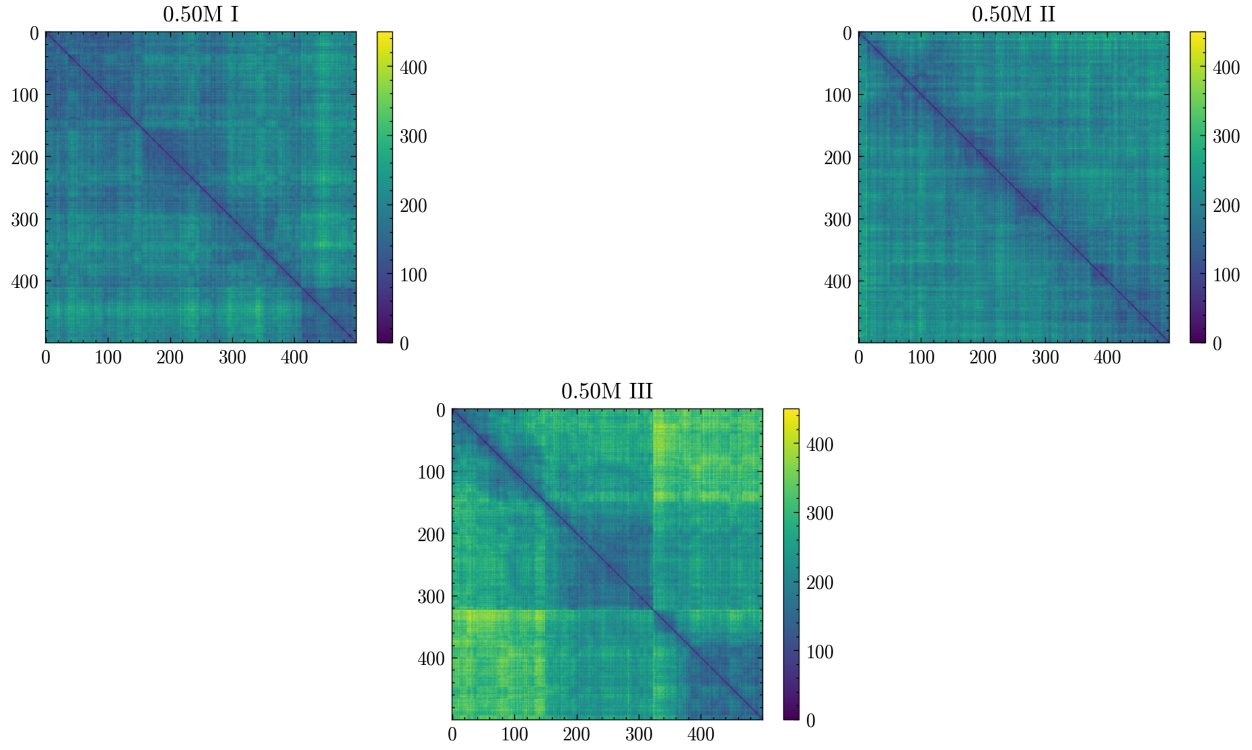


**Supplementary Figure S3**: 2D distance matrices ($d_{KM}$) between contact maps, associated with the freely-folding MD replicas at 0.5 M.

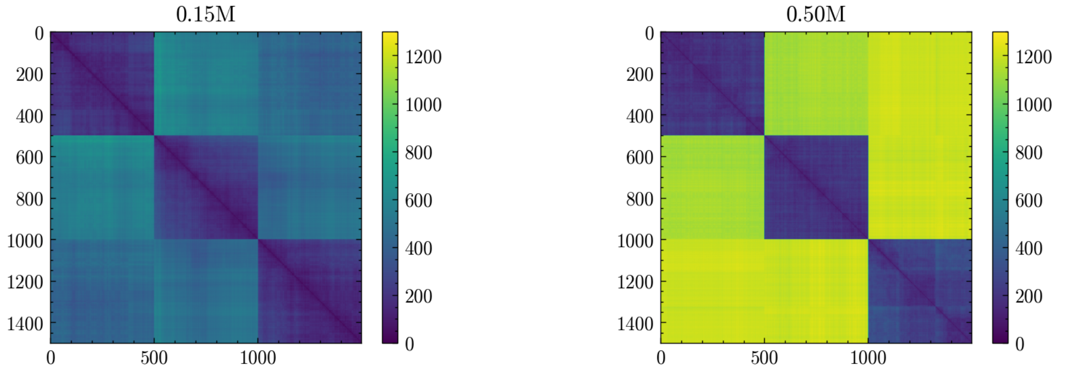


**Supplementary Figure S4**: 2D distance matrices ($d_{KM}$) between contact maps, associated with all frames from all replicas of the freely-folding MD at (**left**) 0.15 M and (**right**) 0.5 M.

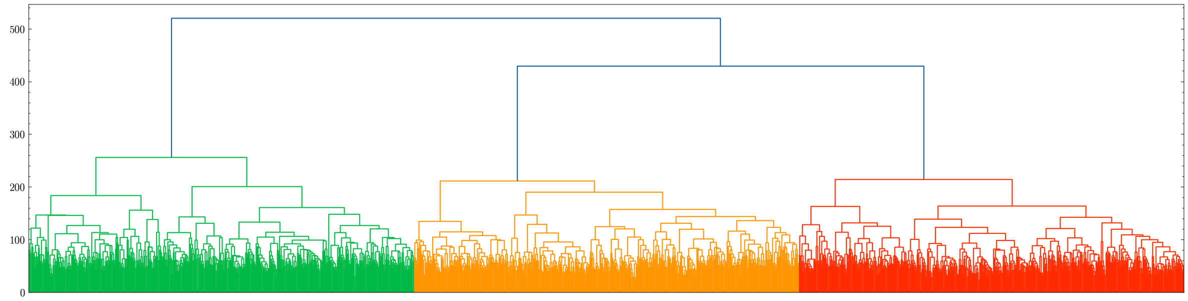


**Supplementary Figure S5**: Dendrogram depiction of the hierarchical clustering of frames from all MD replicas at 0.15 M, based upon the distance between contact maps together with an average linkage criterion: A 1:1 association between MD replicas and clusters highlights the structural dissimilarity between conformational ensembles.

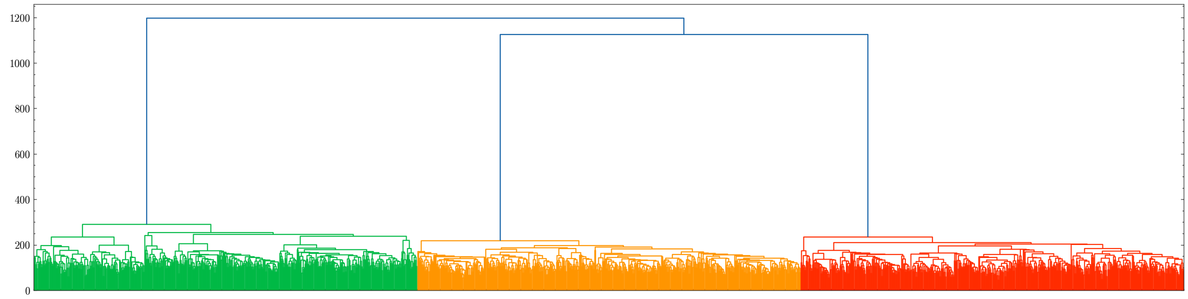


**Supplementary Figure S6**: Dendrogram depiction of the hierarchical clustering of frames from all MD replicas at 0.5 M, based upon the distance between contact maps together with an average linkage criterion: A 1:1 association between MD replicas and clusters highlights the structural dissimilarity between conformational ensembles.

## C. Free energy landscapes

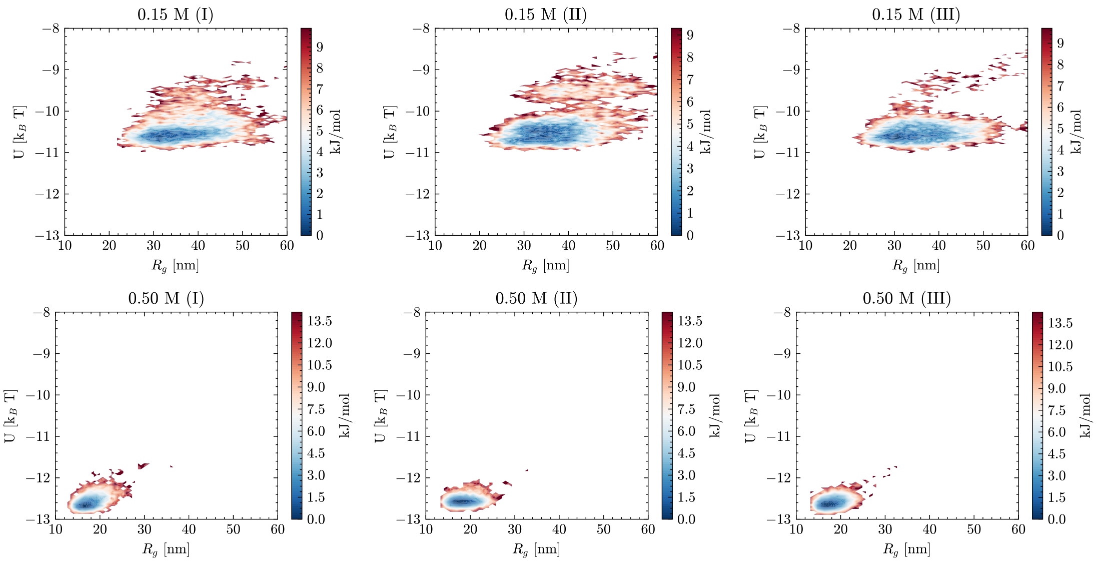


**Supplementary Figure S7**: Free-energy profiles of the RNA2 from the freely-folding MD replicas at (**top**) 0.15 M, and (**bottom**) 0.5 M, based upon the values of the gyration radius ($R_g$) and the internal energy ($U$).

## D. Chord diagram depiction of the stable hydrogen-bonding contacts

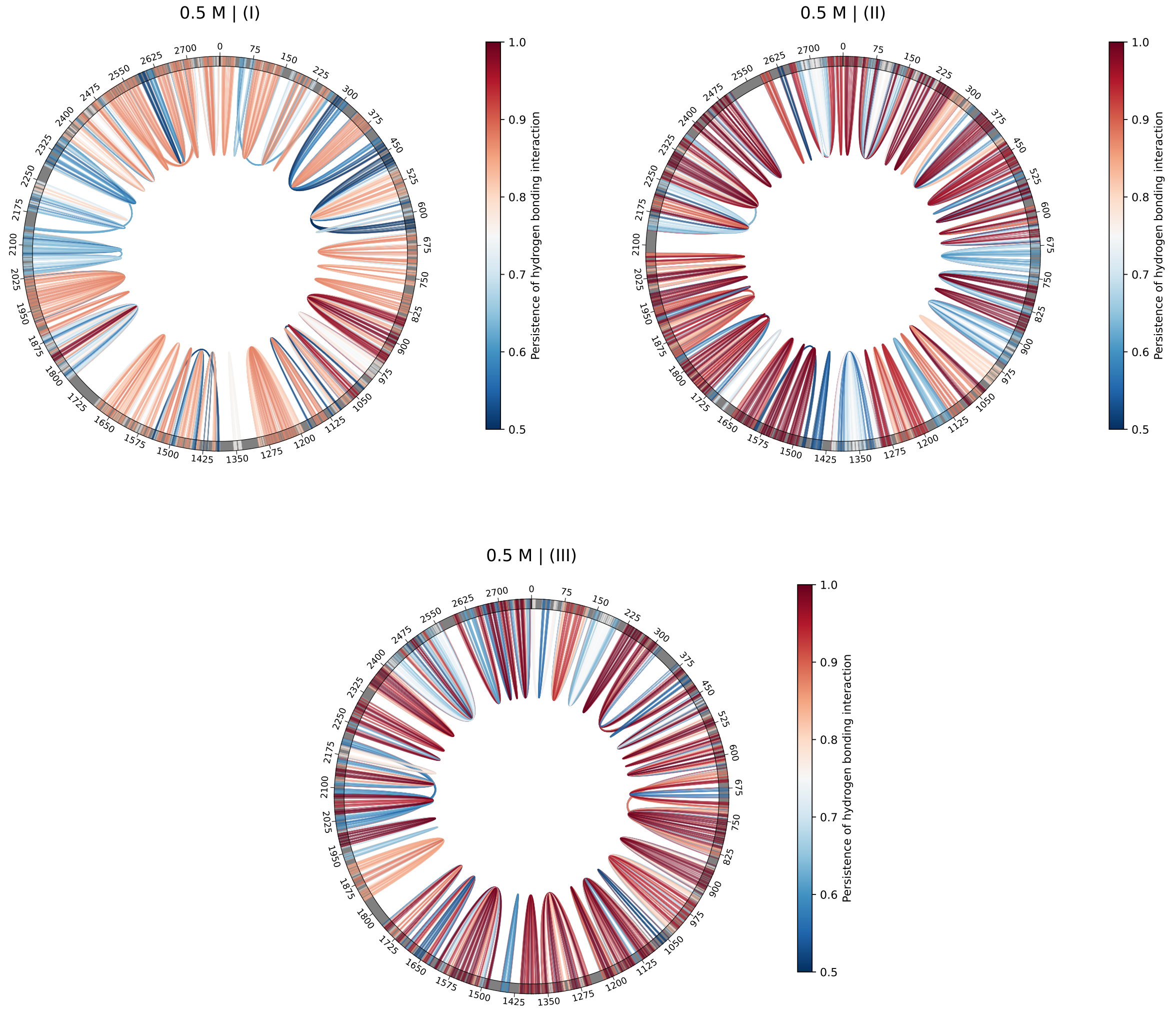


**Supplementary Figure S8**: Chord diagram depiction of the stable hydrogen-bonding contacts, i.e., conserved in over 50% of the trajectory frames, over the equilibrated fraction of (**upper left**) replica I, (**upper right**) replica II, and (**bottom**) replica III of the freely-folding MD at 0.5 M.

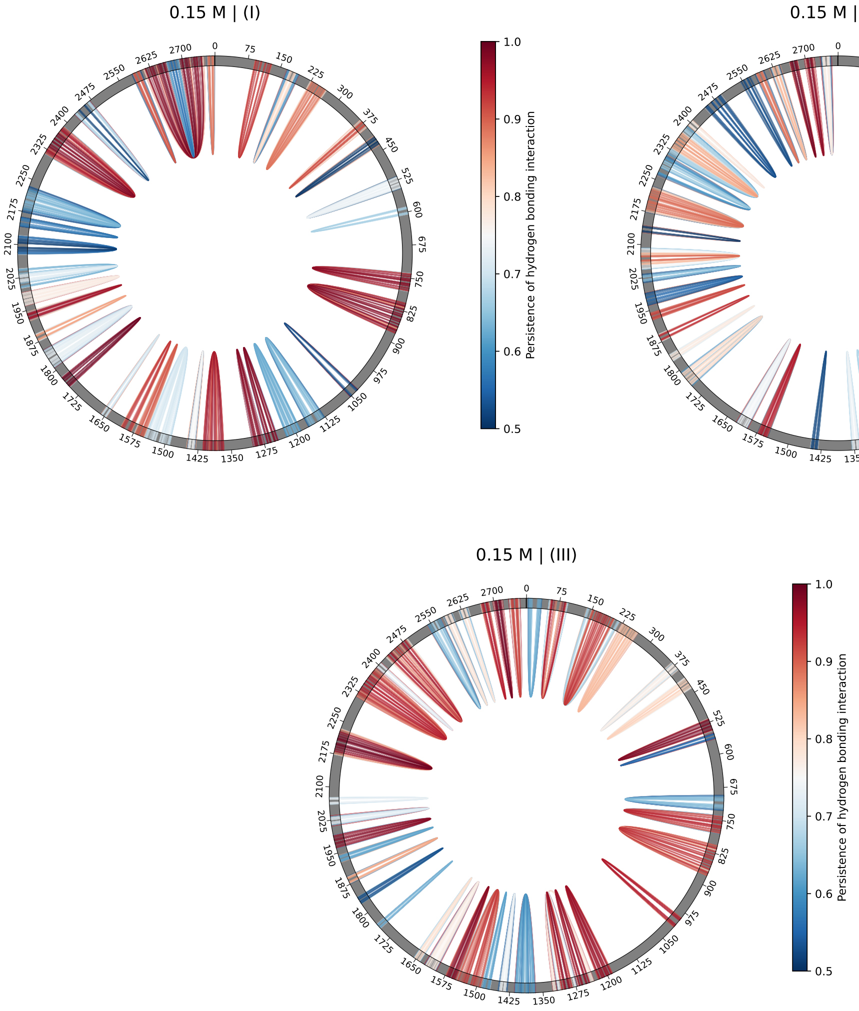


**Supplementary Figure S9**: Chord diagram depiction of the stable hydrogen-bonding contacts, i.e., conserved in over 50% of the trajectory frames, over the equilibrated fraction of (**upper left**) replica I, (**upper right**) replica II, and (**bottom**) replica III of the freely-folding MD at 0.15 M.

## III. ENCAPSIDATION STAGE

### A. Evolution of the internal pressure and of the hydrogen-bonding interactions

We monitored the internal pressure of the RNA2 molecules throughout the encapsidation stage (see Equation **1** in the main text), as effective proxy of a quasi-static transformation. According to this criterion, RNA replicas at 0.5 M were somewhat unaffected by the external force, associated with an encapsidation kinetics of $5.6 \times 10^{-8}$ $\lambda_{ox}$/MD steps (see Figure **S10**) - eventually yielding a spherical volume about 10 nm in radius.
Conversely, the encapsidation of RNA2 at 0.15 M required that a milder kinetics of $1 \times 10^{-8}$ $\lambda_{ox}$/MD steps be applied in the later stage, to keep the internal pressure from diverging - thereby achieving a spherical volume of about 11 nm in radius.

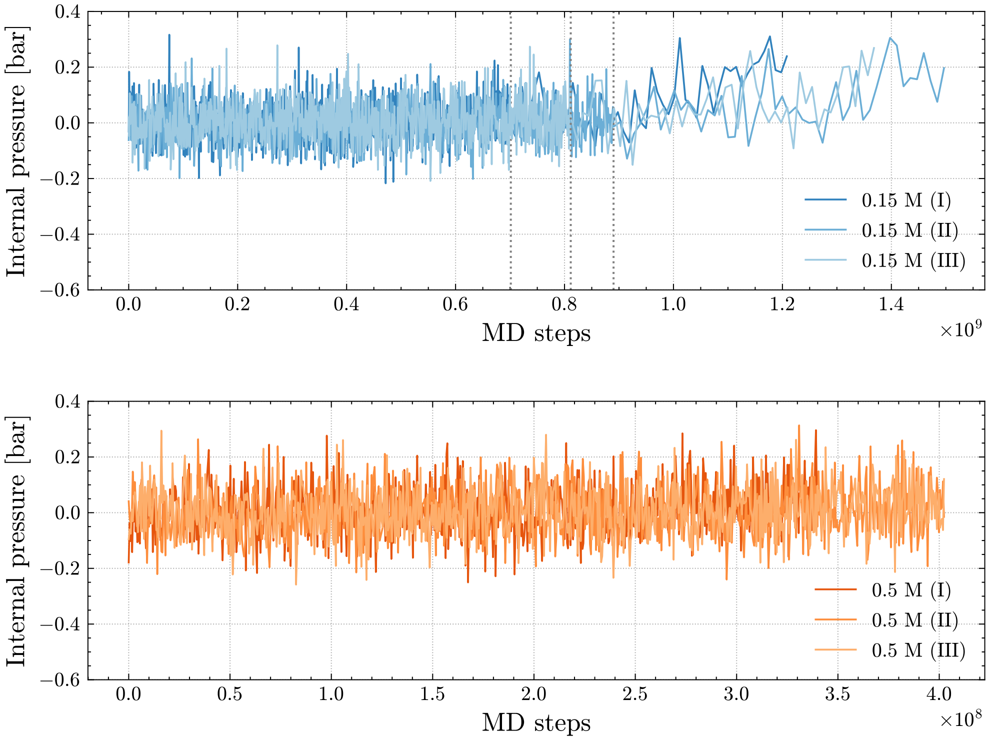


**Supplementary Figure S10**: Estimates of the internal pressure throughout the encapsidation stage of RNA2, at a (**top**) 0.15 M and (**bottom**) 0.5 M concentration of monovalent salt.

Yet, as observed in Figure **S11**, the encapsidation procedure drives a significant rise in the amount of hydrogen-bonding nucleotides - which is steady at 0.5 M and abrupt at 0.15

M, yielding about a 60% contact increase in the latter case. While one might account for this process in terms of spatial proximity, forcibly favouring the pairing of nucleotides, we are inclined to believe this might be an artificial outcome from a strongly non-equilibrium setup.

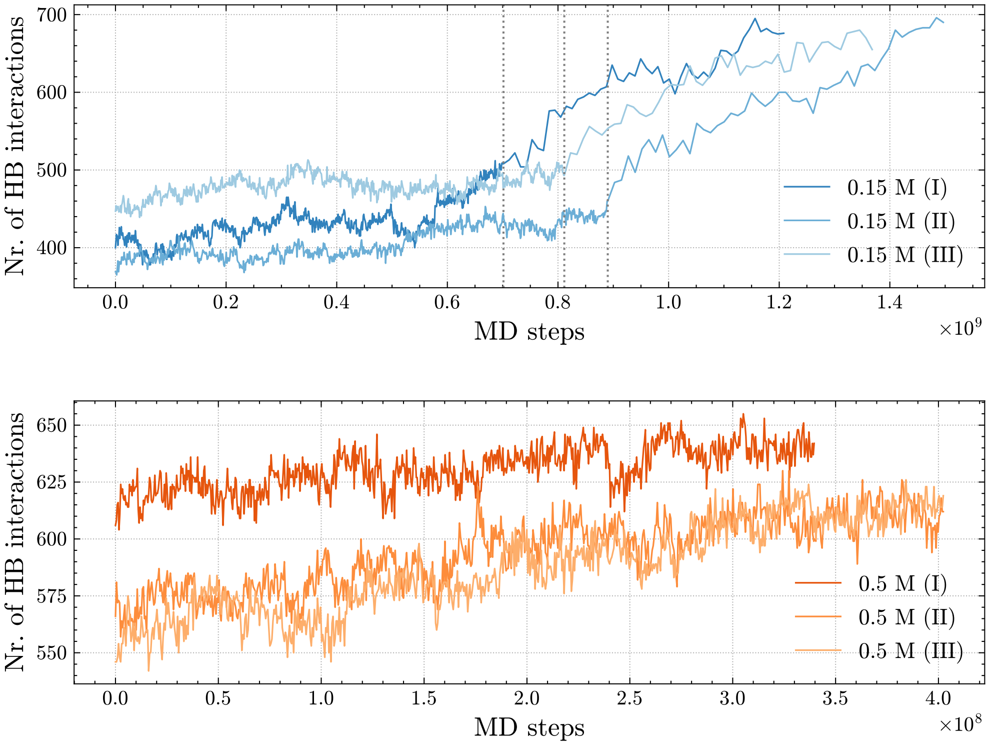


**Supplementary Figure S11**: Evolution of the amount of hydrogen-bonding interactions throughout the encapsidation stage of RNA2 at a (**top**) 0.15 M and (**bottom**) 0.5 M concentration of monovalent salt.

## IV. RNA2 DYNAMICS WITHIN A CCMV CAPSID-LIKE ELECTROSTATIC POTENTIALS

Two mean-field approaches were adopted to the calculation of a radial profile of the electrostatic potential, based upon the theoretical formalism reported by Šiber and Podgornik [1] and atomistic structural data respectively.

### A. Derivation of a spherically-symmetric potential *via* an analytical approach

In Ref. [1], the capsid is depicted as a thin spherical shell of radius $R_0$, associated with a surface charge density $\sigma_c = Q/4\pi R_0^2$. Under the Debye-Hückel approximation of the Poisson-Boltzmann equation, an analytical solution for the electrostatic potential energy (of the internal cavity of the capsid) is thus derived as:

$$U_{theo}(r) = \frac{q_{nuc}\,\beta Q \sinh\left[k_{DH}(R_0 - r)\right]}{4\pi(R_0 - r)\epsilon_0\epsilon_r k_{DH} R_0\{\sinh[k_{DH}(R_0 - r)] + \cosh[k_{DH}(R_0 - r)]\}} \quad (1)$$

with $k_{DH}$ the inverse Debye length, $Q$ the internal charge of the (amino-terminal tails of the) capsomer subunit at physiological pH ($+1800e$), $I = 0.15$ M the monovalent salt concentration, $R_0$ the internal radius of the CCMV capsid (about 12 nm). Here, we set the value of the probe charge $q_{nuc}$ according to the effective charge of the single nucleotide in the oxRNA model.

Figure **S12** shows the outcome of a fitting procedure, whereby we redefined $U_{theo}(r)$ as a combination of a Yukawa (attractive) and WCA (repulsive) potential - refer to the main text for details.

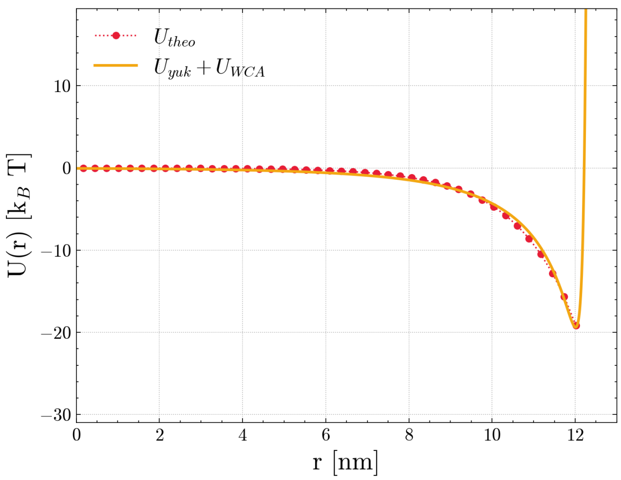


**Supplementary Figure S12**: Plots of the $U_{theo}(r)$ potential energy (red dots) and outcome of the fitting procedure $U_{yuk+WCA}(r)$ (orange solid line) - the latter employed as radial potential profile in the dynamics of RNA2 within a CCMV-like electrostatic field (analytical approach).

## B. Derivation of a capsid-like external field from atomistic data

### *1. Construction of a model capsid structure*

Coordinates of the trimer subunit of the CCMV capsid (chains A, B and C) were obtained from the RCSB Protein Data Bank (entry ID: 1CWP) [2]. The missing residues belonging to the amino-terminal tails of the capsomer subunit (that is, 26 amino acids of chains B and C, and 42 amino acids of chain A) were reconstructed *via* the Chimera visual interface [3] of the Modeller toolkit [4] - whereby the highest-ranking model of five alternative structures was kept.

The newly-achieved subunits were thus subject to a multi-step minimization/equilibration protocol[5], as follows:

1. a first energy minimization of the structure was carried out in vacuum, constraining all atoms of the monomeric subunits **but** the N-terminal tails;

2. the minimized structure was solvated and neutralized by an excess concentration (0.15 M) of sodium chloride;

3. by fixing all atoms of the capsomer subunits **but** the amino-termini, the capsid tails were further minimized and subject to subsequent equilibration steps in the NVT (1 ns) and NPT ensemble (200 ps);

4. from the latter step, we extracted the frame associated with the lowest radius of gyration and carried out a further (restrained) NVT run of $\sim$ 10 ns.

A minimized configuration of the trimeric capsomer is achieved, whereby we selected the coordinates of the monomeric subunit whose amino-terminus interfered the least with the neighboring capsomers. This structure was thus employed to reconstruct the whole CCMV capsid shell (*via* the `MatchMaker` function of Chimera):

1. firstly, by superimposing the subunit to each of the three chains of the trimeric capsomer;

2. hence, by replicating the trimeric capsomer upon the PDB template of the CCMV capsid shell, according to the sixty-fold symmetry of the icosahedral structure

### *2. Energy minimization of the capsid structure and solvent thermalization*

The system topology of the newly-achieved capsid structure was initialized employing the CHARMM36m atomistic force field of biomolecular structures [6] - hence:

1. the capsid was firstly subject to a threefold minimization step in vacuum by a steepest descent algorithm, gradually lowering the force tolerance threshold (5000, 1000 and 100 kJ/(mol nm));

2. the vacuum-minimized system was solvated within a dodecahedral box of TIP3P water molecules and neutralized by an excess (0.15 M) concentration of sodium chloride - likewise, a three-fold minimization protocol was applied;

3. a 10-ps thermal annealing of the solvent bath (i.e., by fixing the coordinates of the CCMV capsid atoms, steadily increasing the temperature to 300 K) was thus performed, followed by a 1-ns thermalization of the solvent bath in the NVT ensemble.

Notably, this protocol yields a significant discontinuity in the radial distribution of the solvent medium, at the core of the capsid shell (as shown by Figure **S13**), despite the

simulation showing no numerical instability. In fact, a similar artifact was observed earlier by Freddolino and co-workers [7], likely accounted for by a (slowly-equilibrating) mismatch between the density of the physiological medium (from the solvation routine) and that of the target system.

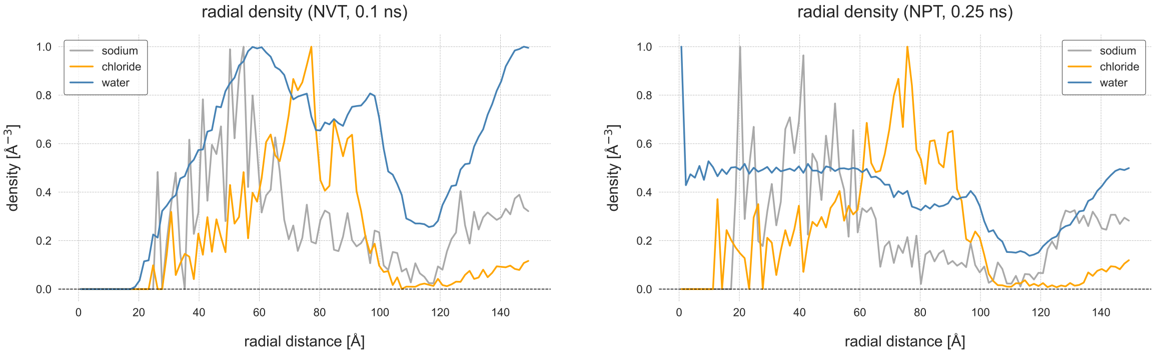


**Supplementary Figure S13**: Radial density profile of the solvent medium (**left**) after the first 100-ps thermalization in the NVT ensemble - highlighting the void at the core of the simulation box; (**right**) after the re-equilibration protocol (detail in the text). For the benefit of clarity, all values are normalized to 1.

The void was thus aptly filled *via* a further solvation step, and the capsid structure subsequently re-equilibrated by i) $<$ 9000 steepest-descent, minimization steps (force threshold: 1000 kJ/mol nm); ii) a 500-ps solvent thermalization in the NVT ensemble; iii) a 250-ps density equilibration in the NPT ensemble.

#### *3. Derivation of a radial potential profile from the atomistic structure of CCMV via Gauss' theorem*

The distribution of the (partial) charges from the last frame of the MD minimization/thermalization protocol (described in Section IV B 2 - see Figure **S14**) was adopted in the calculation of a mean-field, radial electrostatic potential associated with the CCMV capsid and the electrolyte distribution thereof.

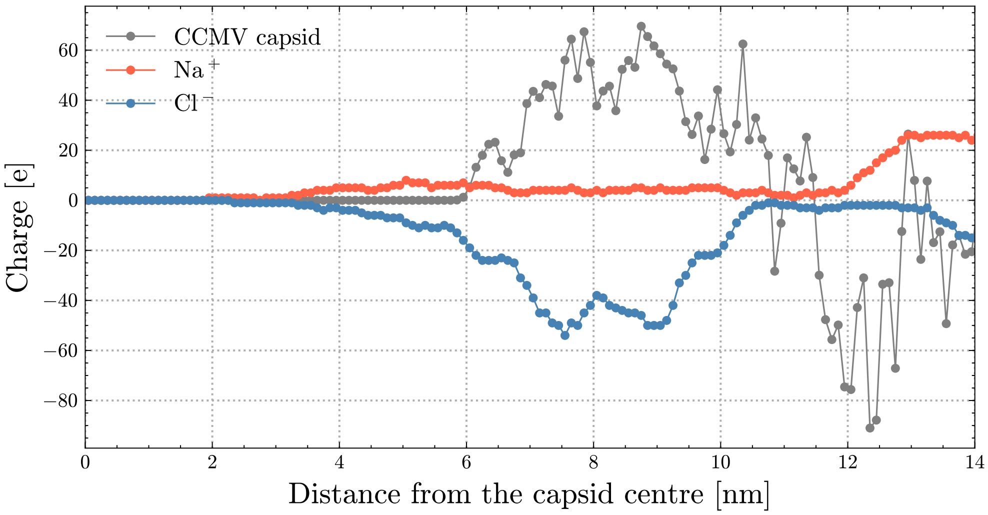


**Supplementary Figure S14**: Profiles of the radial charge distribution associated with the CCMV capsid and the ionic shells thereof, from the last frame of the MD minimization/thermalization protocol described in Section IV B 2. Contributions from each species are integrated over 1 Å-thick spherical shells, along the radial distance from the core of the capsid.

The calculation requires that the charge distribution be firstly discretized along the radial distance as $\rho(r) \approx \rho[r_i] \equiv \rho_i$, with $i$ denoting a binning interval $I_i = \left[ r_i - \frac{\delta R}{2}, r_i + \frac{\delta R}{2} \right]$ of thickness $\delta R = 1$ Å.

By assuming $\rho_i$ to be spherically-symmetric, we define the charge density of the $i$-th shell as:

$$\rho_i = \frac{Q_i}{\frac{4}{3}\pi \left( \left( r_i + \frac{\delta R}{2} \right)^3 - \left( r_i - \frac{\delta R}{2} \right)^3 \right)} \equiv \frac{Q_i}{\frac{4}{3}\pi \delta R \left( 3r_i^2 + \frac{(\delta R)^2}{4} \right)}, \tag{2}$$

with $Q_i$ the total (net) charge from the contributions of all species within interval $I_i$.

Within the approximation of spherical symmetry, the radial electric field (i.e. $\mathbf{E}(\mathbf{r}) = E(r)\hat{r}$) originated by a charged shell of volume $\mathcal{V}_i$ and total charge $Q_i = \rho_i \mathcal{V}_i$ is straightforwardly derived *via* Gauss' theorem:

$$E_i(r) = \begin{cases} 0, & \text{if } r < r_i \\ \frac{Q_i}{4\pi\epsilon_0 r^2}, & \text{if } r \geq r_i. \end{cases} \tag{3}$$

Hence, the electric potential $V(r)$:

$$V(r) - V(\infty) := -\int_r^\infty dr'\ E(r') = \begin{cases} 0, & \text{if } r < r_i \\ \dfrac{Q_i}{4\pi\epsilon_0 r}, & \text{if } r \geq r_i \end{cases} \tag{4}$$

with $V(\infty)$ set to zero. Each shell $I_i$ is thus subject to the electric field enforced by all layers underneath, so that at a radial distance $R_i$:

$$V(R_i) - V(\infty) := -\int_{R_i}^\infty dr' \left( \sum_{j=1}^{i} E_j(r') \right) \tag{5}$$

thereby obtaining a discretized version of $V_{cap}(r)$, denoted $V_{cap}[r]$. To convert this mean-field potential into an electric potential energy $U_{cap}[r] = qV[r]$, we employed a probe charge $q = q_{nuc}$ corresponding to the effective charge of the single nucleotide adopted in the oxRNA model. A Gaussian-filtered version of the electric potential energy $U_{cap}[r]$, denoted $\tilde{U}_{cap}[r]$, was fitted by a polynomial curve - as described in the main text: This expression ($U_{cap}(r)$) was lastly implemented within the oxDNA code.

### C. Fitting parameters

#### 1. *Analytical approach*

Here is a list of the parameters derived from the fitting procedure of the analytical solution reported by Šiber and Podgornik [1] (Equation **2** of the main article):

- $\alpha = -4.3\ k_BT$
- $\lambda = 3.448\ \lambda_{ox}$ the Debye length,
- $\epsilon = 1 \times 10^{-4}\ k_BT$
- $\sigma = 1.9\ \lambda_{ox}$
- $R_\delta := R_0 + \delta = 15.5\ \lambda_{ox}$ , to avoid divergences of the forces acting on particles close to the surface in $R_0$.

#### 2. *Structure-based approach*

Here is a list of the parameters derived from the fitting procedure of the discredited potential energy $U_{cap}(r)$, obtained from the atomistic structures of the CCMV capsid as described in Section IV B 3 (Equation **3** of the main article).

- $R_0 = 14.8\ \lambda_{ox}$
- $A = -7.77913022 \times 10^{-2}\ k_BT/\lambda_{ox}$
- $c_1 = 4.59994536\ \lambda_{ox}^{-1}$
- $c_2 = -1.08939804 \times 10^{1}\ \lambda_{ox}^{-2}$
- $c_3 = 7.68423122\ \lambda_{ox}^{-3}$
- $c_4 = -2.79192908\ \lambda_{ox}^{-4}$
- $c_5 = 6.06976204 \times 10^{-1}\ \lambda_{ox}^{-5}$
- $c_6 = -8.29137297 \times 10^{-2}\ \lambda_{ox}^{-6}$

- $c_7 = 7.15232653e \times 10^{-3}\ \lambda_{ox}^{-7}$
- $c_8 = -3.77388959 \times 10^{-4}\ \lambda_{ox}^{-8}$
- $c_9 = 1.11053305 \times 10^{-5}\ \lambda_{ox}^{-9}$
- $c_{10} = -1.39522295 \times 10^{-7}\ \lambda_{ox}^{-10}$

### D. Internal energy and pressure of the RNA2 molecules

Values of the internal energy and pressure of the RNA2 molecules in the two external field scenarios are shown in Fig. **S15** and **S16** respectively. Although the latter are somewhat equivalent, the analytical protocol shows higher values of the internal energy - arguably on account of the disruption of hydrogen-bonding interactions and secondary structures.

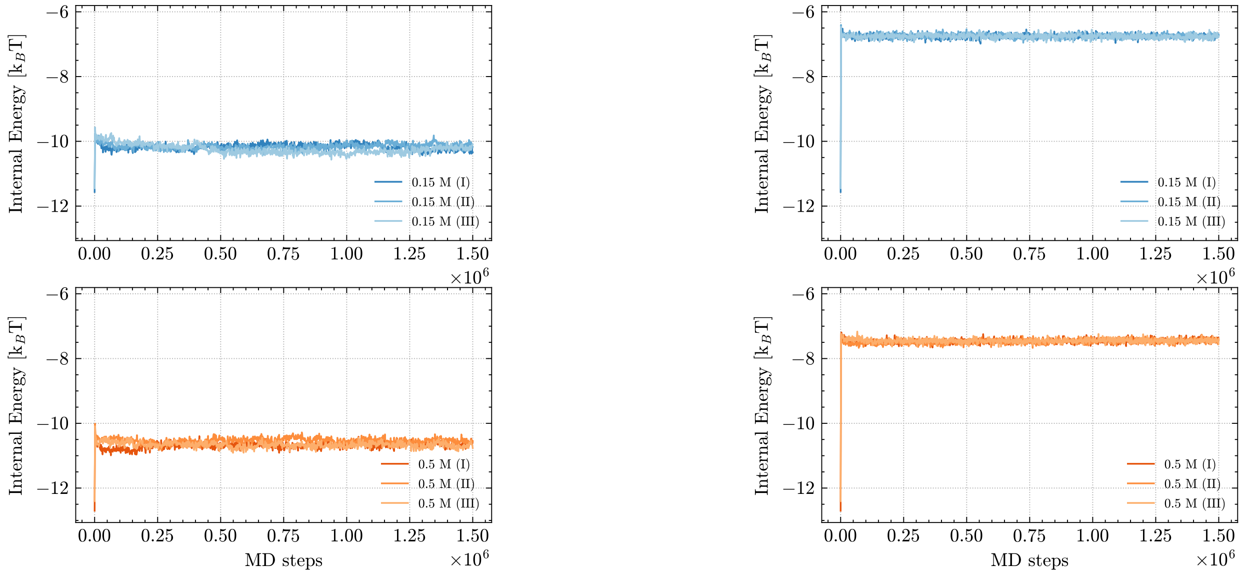


**Supplementary Figure S15**: Values of the internal energy of the RNA2 molecules, for the MD replicas associated with the **(left)** structure-based, and **(right)** analytical approach.

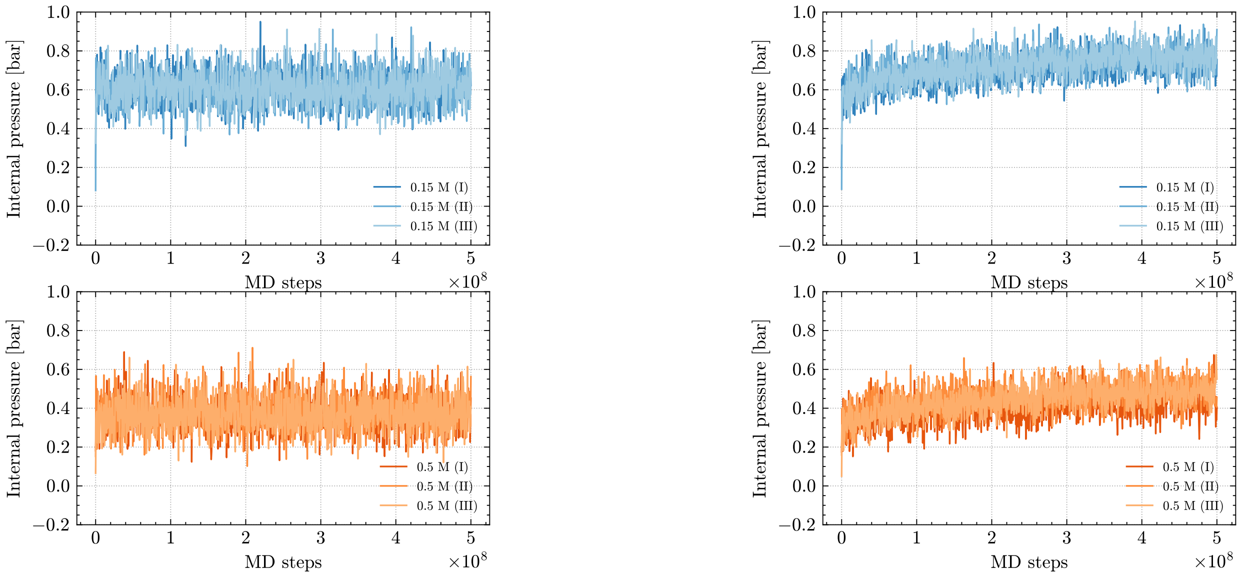


**Supplementary Figure S16**: Values of the internal pressure of the RNA2 molecules, for the MD replicas associated with the **(left)** structure-based, and **(right)** analytical approach.

### E. Chord diagram depiction of the stable hydrogen-bonding contacts

#### *1. Chord diagrams associated with each independent replica in the structure-based approach*

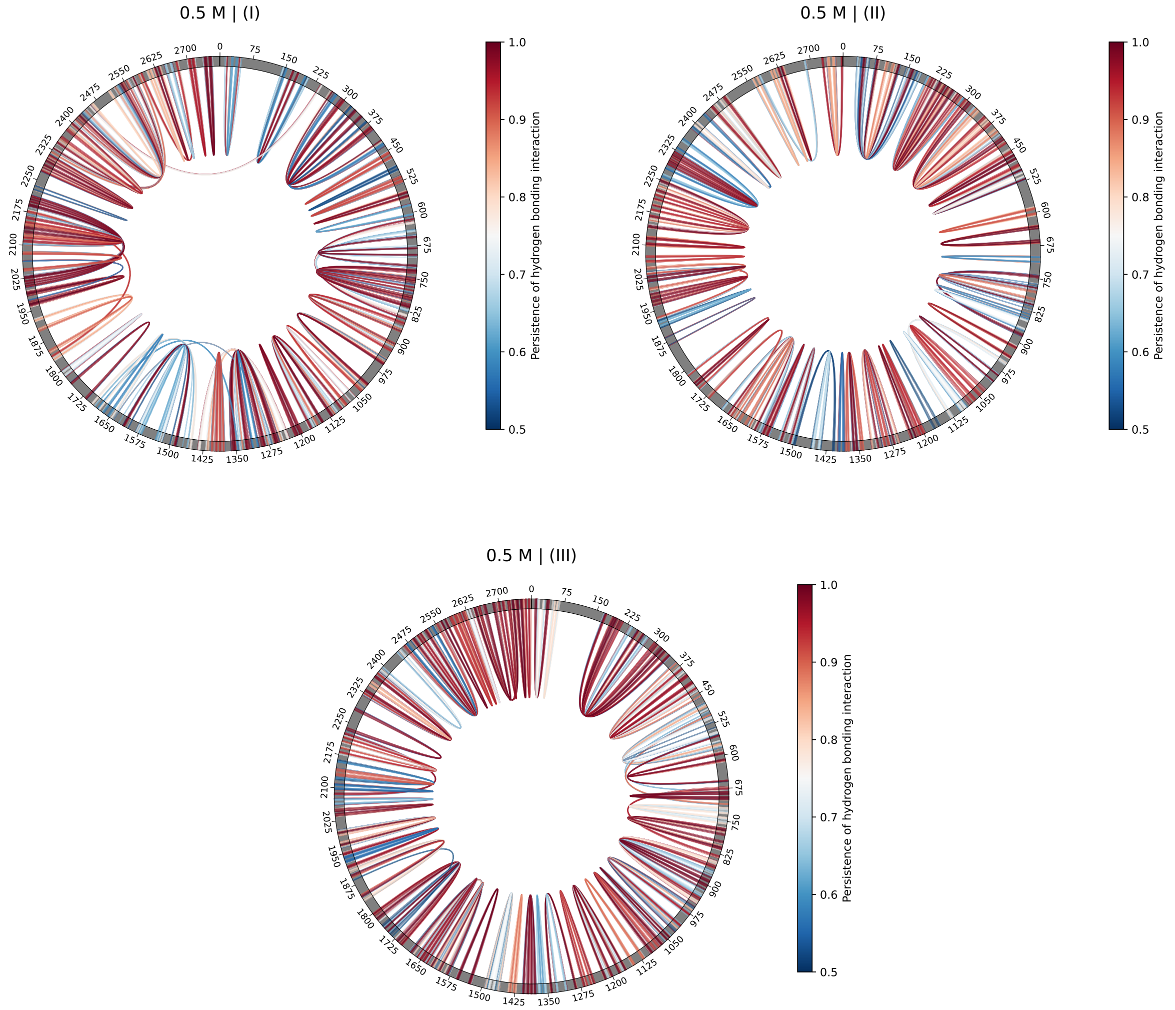


**Supplementary Figure S17**: Chord diagram depiction of the stable hydrogen-bonding contacts, i.e., conserved in over 50% of the trajectory frames, within (**upper left**) replica I, (**upper right**) replica II, and (**bottom**) replica III, at 0.5 M - data shown here refer to the structure-based approach.

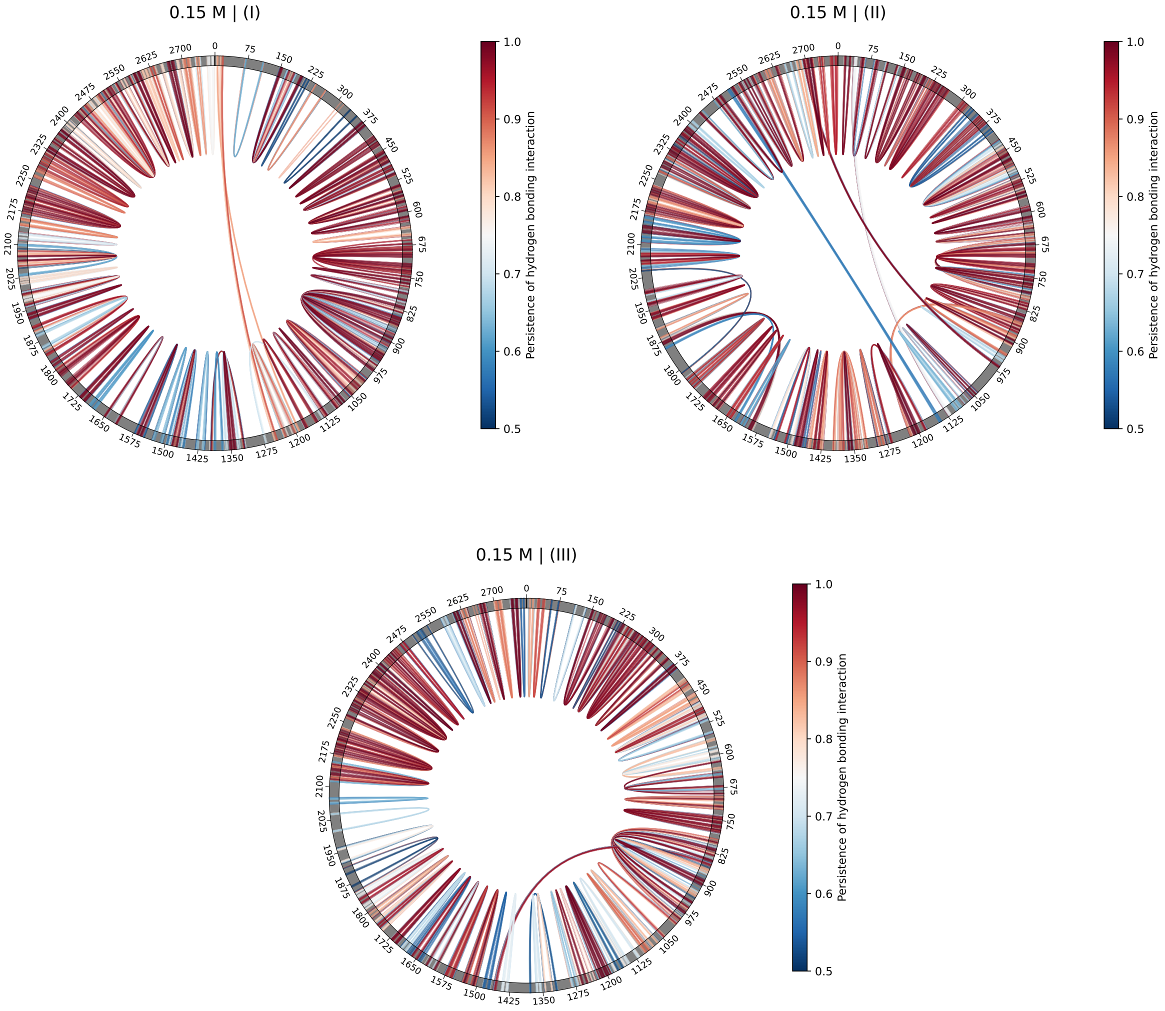


**Supplementary Figure S18**: Chord diagram depiction of the stable hydrogen-bonding contacts, i.e., conserved in over 50% of the trajectory frames, within (**upper left**) replica I, (**upper right**) replica II, and (**bottom**) replica III, at 0.15 M - data shown here refer to the structure-based approach.

*2. Chord diagrams associated with an averaging procedure over the independent MD replicas in the structure-based approach*

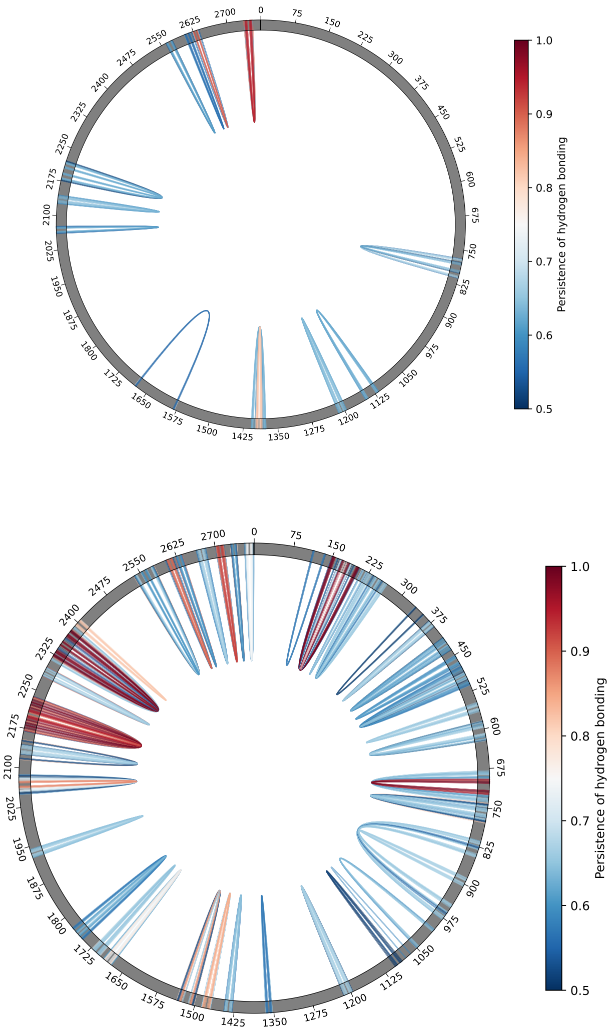


**Supplementary Figure S19**: Chord diagram depiction of the stable hydrogen-bonding contacts (i.e., conserved in over 50% of the total trajectory frames per salt concentration), from the structure-based approach at (left) 0.5 M and (right) 0.15 M

[1] A. Šiber and R. Podgornik, Role of electrostatic interactions in the assembly of empty spherical viral capsids, Physical Review E—Statistical, Nonlinear, and Soft Matter Physics **76**, 061906 (2007).

[2] J. A. Speir, S. Munshi, G. Wang, T. S. Baker, and J. E. Johnson, Structures of the native and swollen forms of cowpea chlorotic mottle virus determined by x-ray crystallography and cryo-electron microscopy, Structure **3**, 63 (1995).

[3] E. F. Pettersen, T. D. Goddard, C. C. Huang, G. S. Couch, D. M. Greenblatt, E. C. Meng, and T. E. Ferrin, Ucsf chimera—a visualization system for exploratory research and analysis, Journal of computational chemistry **25**, 1605 (2004).

[4] A. Fiser and A. Šali, Modeller: generation and refinement of homology-based protein structure models, in *Methods in enzymology*, Vol. 374 (Elsevier, 2003) pp. 461–491.

[5] All minimization and equilibration steps hereby described were carried out *via* the 2018 version of the Gromacs toolkit [8].

[6] J. Huang, S. Rauscher, G. Nawrocki, T. Ran, M. Feig, B. L. De Groot, H. Grubmüller, and A. D. MacKerell Jr, Charmm36m: an improved force field for folded and intrinsically disordered proteins, Nature methods **14**, 71 (2017).

[7] P. L. Freddolino, A. S. Arkhipov, S. B. Larson, A. McPherson, and K. Schulten, Molecular dynamics simulations of the complete satellite tobacco mosaic virus, Structure **14**, 437 (2006).

[8] M. J. Abraham, T. Murtola, R. Schulz, S. Páll, J. C. Smith, B. Hess, and E. Lindahl, Gromacs: High performance molecular simulations through multi-level parallelism from laptops to supercomputers, SoftwareX **1**, 19 (2015).
